# Supplementary material for: Persistence of charge ordering instability to Coulomb engineering in the excitonic insulator candidate TiSe$_2$
Source: arXiv:2506.01470 source file (2025-06-02)
Supplement: Supplementary file 1 [file supp.pdf]

# Supplementary Information: Persistence of charge ordering instability to Coulomb engineering in the excitonic insulator candidate $TiSe_2$

Sebastian Buchberger,[1,2] Yann in 't Veld,[3] Akhil Rajan,[1] Philip A. E. Murgatroyd,[1] Brendan Edwards,[1] Bruno K. Saika,[1] Naina Kushwaha,[1,4] Maria H. Visscher,[1,2] Jan Berges,[5] Dina Carbone,[6] Jacek Osiecki,[6] Craig Polley,[6] Tim Wehling,[3,7,*] and Phil D. C. King[1,†]

[1] *SUPA, School of Physics and Astronomy, University of St Andrews, St Andrews KY16 9SS, United Kingdom*
[2] *Max Planck Institute for Chemical Physics of Solids, Nöthnitzer Strasse 40, D-01187 Dresden Germany*
[3] *I. Institute of Theoretical Physics, Universität Hamburg, D-22607 Hamburg, Germany*
[4] *STFC Central Laser Facility, Research Complex at Harwell, Harwell Campus, Didcot OX11 0QX, United Kingdom*
[5] *U Bremen Excellence Chair, Bremen Center for Computational Materials Science, and MAPEX Center for Materials and Processes, University of Bremen, D-28359 Bremen, Germany*
[6] *MAX IV Laboratory, Lund University, Lund, Sweden*
[7] *The Hamburg Centre for Ultrafast Imaging, D-22761 Hamburg, Germany*

(Dated: May 31, 2025)

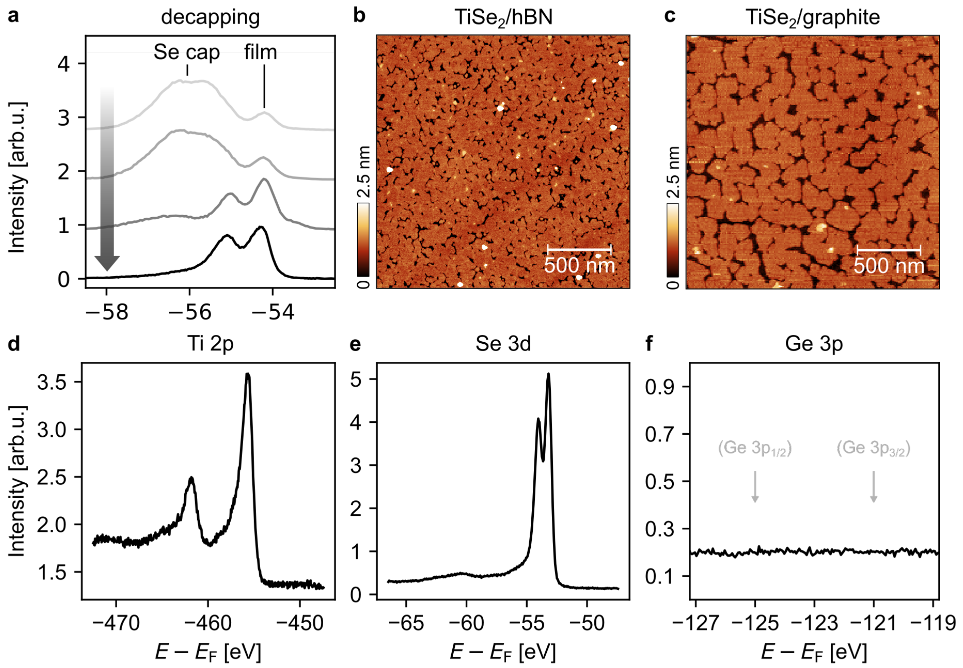


Supplementary Fig. 1. Material characterisation of monolayer $TiSe_2$ samples. (a) Se 3d XPS peaks monitored while optimising the Se decapping procedure. The arrow indicates the sequence of decapping iterations. A broad set of peaks corresponding to the amorphous Se cap monotonously decreases with each iteration, leaving a narrower, clean doublet for the completely decapped sample. (b,c) AFM measurements of $TiSe_2$/hBN and $TiSe_2$/graphite sister samples of the samples measured in the main manuscript, showing high monolayer coverage and negligible bilayer formation. (d–f) XPS measurements measured atop an hBN flake after decapping at the Bloch endstation. Clear Ti 2p and Se 3d core levels from the $TiSe_2$ film are present. No signal corresponding to Ge is visible, demonstrating that no detectable amount of Ge is incorporated in the film from our nucleation-assisted growth procedure [1].

* Correspondence to: tim.wehling@physik.uni-hamburg.de
† Correspondence to: pdk6@st-andrews.ac.uk

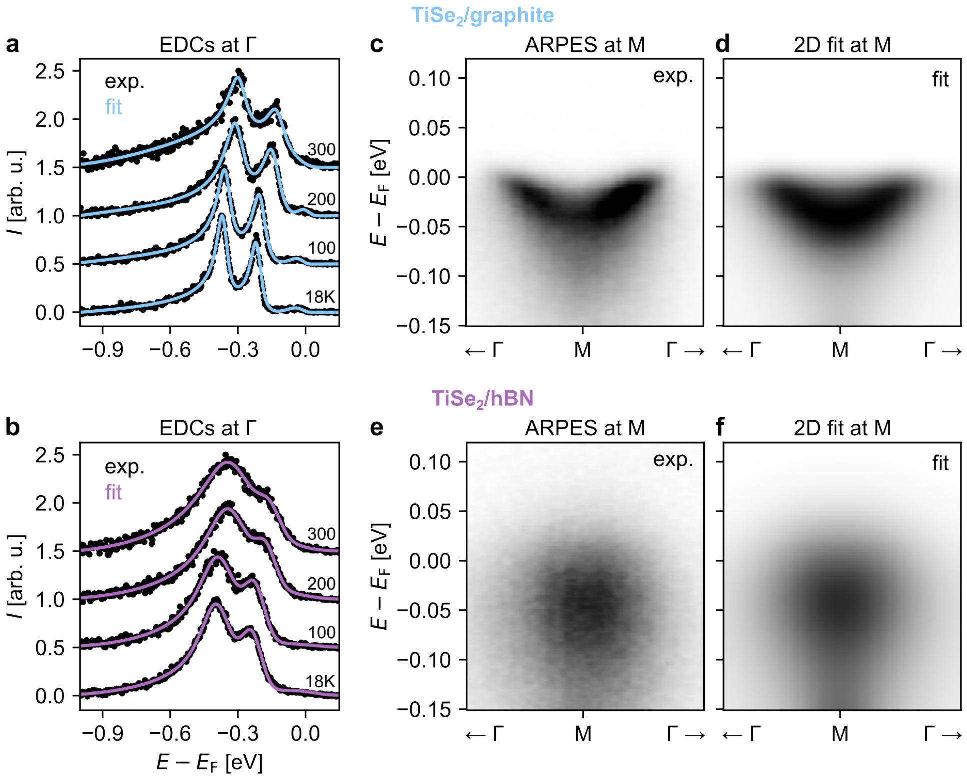


Supplementary Fig. 2. Fitting of valence and conduction band of $TiSe_2$ on graphite and hBN. (a,b) One-dimensional fits to EDCs at the Γ point from $TiSe_2$/graphite ((a), top) and $TiSe_2$/hBN ((b), bottom) for selected temperatures. (c–f) ARPES data (c,e) and two-dimensional fits (d,f) of the Ti 3d conduction band for $TiSe_2$/graphite (c,d) and $TiSe_2$/hBN (e,f), respectively. For the two-dimensional fitting of the spectral function, the underlying model assumes a parabolic bare band dispersion, a constant imaginary part of the self energy, a Fermi cut-off, and Gaussian broadening in energy and momentum. Note that the contrast in (e) and (f) is enhanced to show the conduction band tail clearly for $TiSe_2$/hBN. The intensity of the measured $TiSe_2$ conduction band is in reality several times lower for $TiSe_2$/hBN as compared to $TiSe_2$/graphite when normalised to the corresponding valence band intensity, reflecting that the conduction band is essentially unoccupied for the former.

[1] A. Rajan, S. Buchberger, B. Edwards, A. Zivanovic, N. Kushwaha, C. Bigi, Y. Nanao, B. K. Saika, O. R. Armitage, P. Wahl, P. Couture, and P. D. C. King, Epitaxial growth of large-area monolayers and van der waals heterostructures of transition-metal chalcogenides via assisted nucleation, Advanced Materials **36**, 2402254 (2024).

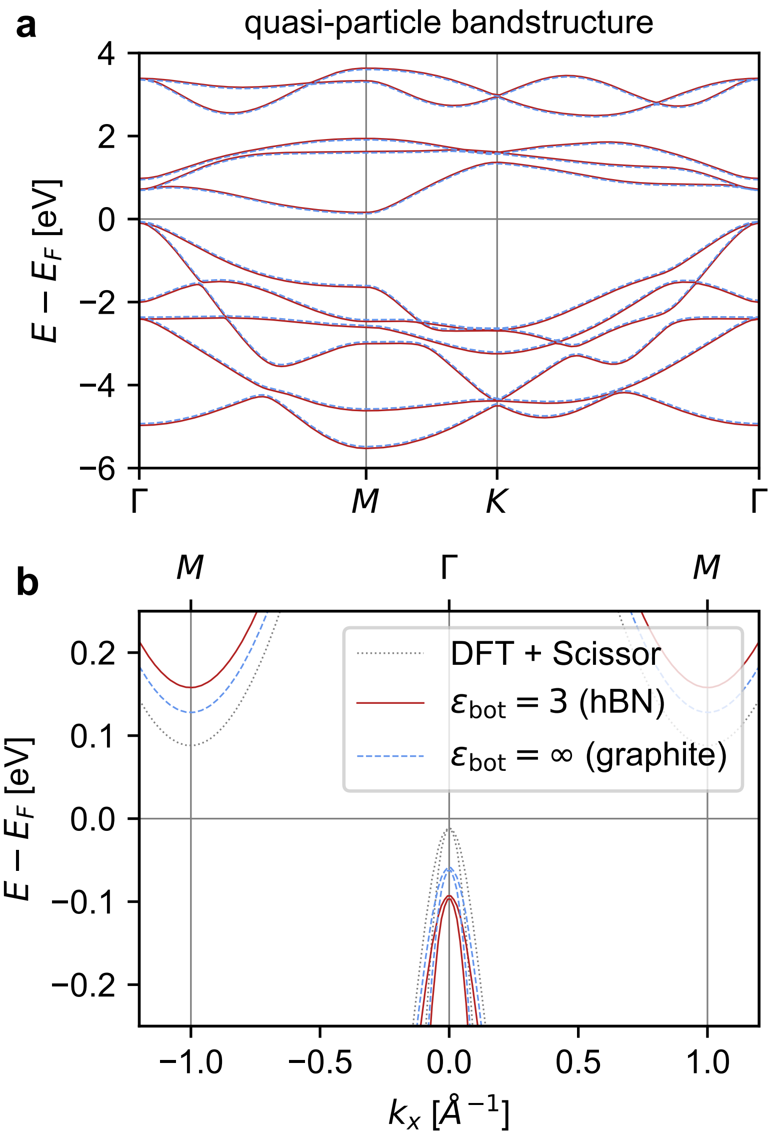


Supplementary Fig. 3. Calculations of band-gap renormalization. (a) Quasi-particle band structure in the COHSX approximation for ML-$TiSe_2$/hBN (red solid line, $\varepsilon_{\rm bot} = 3$) and ML-$TiSe_2$/graphite (blue dashed line, $\varepsilon_{\rm bot} = \infty$) along two different paths in the first Brillouin zone, with a magnified view around the band gap shown in (b). In (b), we also show the bare DFT bandstructure after including a gap with the scissor operator (gray dotted line, see Appendix in the main text).

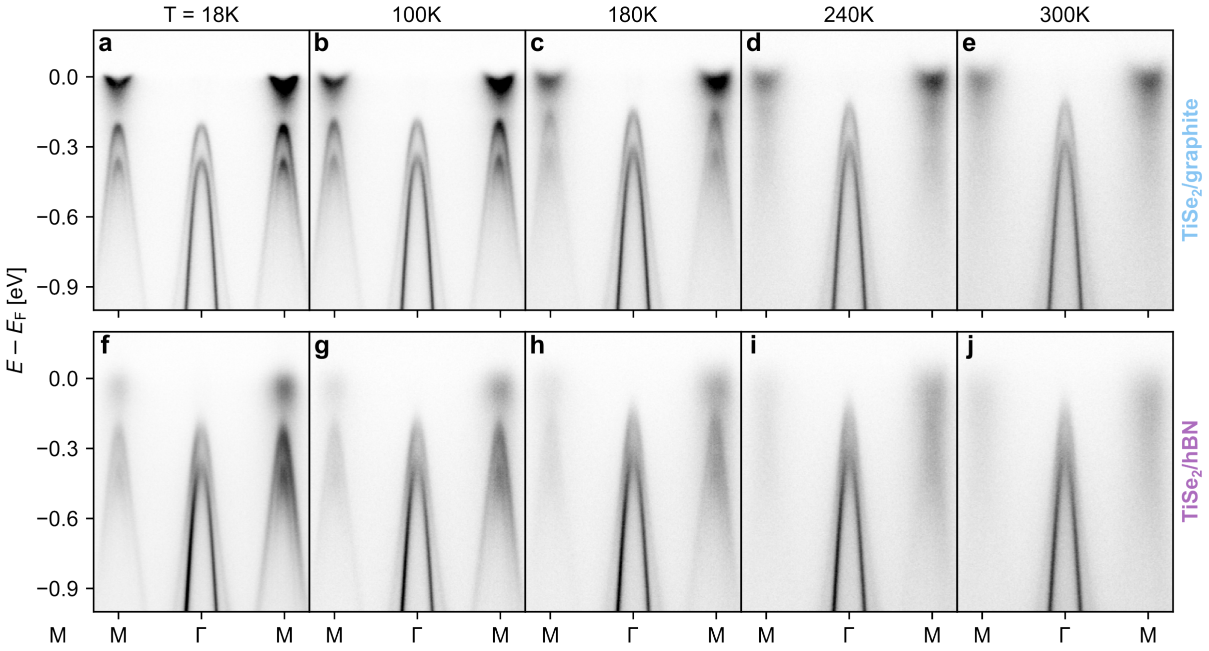


Supplementary Fig. 4. Temperature-dependent electronic structure. Temperature-dependent ARPES spectra of ML-$TiSe_2$/graphite ((a–e), top row) and ML-$TiSe_2$/hBN ((f–j), bottom row).
